# Supplementary material for: Isotopic and vibrational-level dependence of H$_2$ dissociation by electron impact
Source: arXiv:2011.12607 ancillary file (2020-11-25)
Supplement: Supplementary file 1 [file supplementary_material.pdf]

# Supplementary material for: "Isotopic and vibrational-level dependence of $H_2$ dissociation by electron impact"

Liam H. Scarlett[1], Dmitry V. Fursa[1], Jack Knol[1], Mark C. Zammit[2], and Igor Bray[1]
[1] *Curtin Institute for Computation and Department of Physics and Astronomy, Curtin University, Perth, Western Australia 6102, Australia and*
[2] *Theoretical Division, Los Alamos National Laboratory, Los Alamos, New Mexico 87545, USA*
(Dated: November 21, 2020)

**This document provides supplementary information to the paper titled "Isotopic and vibrational-level dependence of $H_2$ dissociation by electron impact".**

Here we provide a corrected derivation of the adiabatic-nuclei (AN) dissociation cross section, following the same ideas laid out by Trevisan and Tennyson [1] (TT01). We use SI units throughout to enable easy comparison with the equations given by TT01. Rather than treating rotational motion explicitly, TT01's derivation assumes a fixed nuclear orientation during the collision and then applies a classical orientation-averaging technique. This approach is valid and formally equivalent to summing over final rotational levels [2]. With the orientation fixed we remove the nuclear orientation $\hat{\boldsymbol{R}}$ from the set of dynamical variables and treat the nuclear motion as a purely one-dimensional problem.

Standard quantum mechanics texts, such as Sakurai and Napolitano [3], derive expressions for the scattering transition rate. For the present case we can write it as

$$w_{i\to f} = \frac{2\pi}{\hbar}\left|T_{f,i}\right|^2 \rho_{\mathrm{e}}(E_{\mathrm{out}},\Omega)\rho_{\mathrm{v}}(E_{\mathrm{k}})\,\mathrm{d}E_{\mathrm{out}}\,\mathrm{d}\Omega, \tag{1}$$

where $E_{\mathrm{out}}$ and $\Omega$ are the scattered electron energy and direction, $E_{\mathrm{k}}$ is the asymptotic kinetic energy of the dissociating fragments, and $\rho_{\mathrm{v}}$ and $\rho_{\mathrm{e}}$ are the states for the target vibrational continuum and scattered electron continuum, respectively. Here, $T_{f,i}$ is the $T$-matrix element linking the final and initial scattering states:

$$T_{f,i} = \langle \nu_{E_{\mathrm{k}}}\boldsymbol{p}_f\Phi_f|\mathbf{T}|\Phi_i\nu_v\boldsymbol{p}_i\rangle \tag{2}$$

where $\boldsymbol{p}_f$ and $\boldsymbol{p}_i$ are the final and initial projectile plane waves, $\nu_{E_{\mathrm{k}}}$ is the continuum vibrational wave function for the dissociating fragments, $\nu_v$ is the bound vibrational wave function for initial level $v$, and $\Phi_f$ and $\Phi_i$ are the final and initial electronic states. Note that Eq. (1) assumes the $\mathbf{T}$ operator is defined by [3]

$$\mathbf{S} = \mathbf{1} - 2\pi i\mathbf{T}. \tag{3}$$

We use the standard momentum-normalized plane waves for the incident and scattered electrons

$$\langle \boldsymbol{r}|\boldsymbol{p}\rangle = \frac{1}{(2\pi\hbar)^{3/2}}e^{i\boldsymbol{p}\cdot\boldsymbol{r}/\hbar} \tag{4}$$

$$\int_{\mathbb{R}^3}\langle \boldsymbol{p}'|\boldsymbol{r}\rangle\langle\boldsymbol{r}|\boldsymbol{p}\rangle\,\mathrm{d}\boldsymbol{r} = \delta(\boldsymbol{p}'-\boldsymbol{p}), \tag{5}$$

which implies the following unity resolution:

$$\int_{\mathbb{R}^3}\langle \boldsymbol{r}'|\boldsymbol{p}\rangle\langle\boldsymbol{p}|\boldsymbol{r}\rangle\,\mathrm{d}\boldsymbol{p} = \delta(\boldsymbol{r}'-\boldsymbol{r}), \tag{6}$$

and incident current density

$$j_i = \frac{\hbar k_i}{m_{\mathrm{e}}(2\pi\hbar)^3}. \tag{7}$$

According to standard definitions [3], the cross section $\mathrm{d}\sigma$ associated with the transition rate (1) is

$$\begin{aligned}\mathrm{d}\sigma &= \frac{w}{j_i}\\ &= \frac{\hbar m_{\mathrm{e}}(2\pi)^4}{k_i}\left|T_{f,i}\right|^2\rho_{\mathrm{e}}(E_{\mathrm{out}},\Omega)\rho_{\mathrm{v}}(E_{\mathrm{k}})\,\mathrm{d}E_{\mathrm{out}}\,\mathrm{d}\Omega,\end{aligned} \tag{8}$$

and hence the double differential cross section (DDCS) is

$$\frac{\mathrm{d}^2\sigma}{\mathrm{d}E_{\mathrm{out}}\,\mathrm{d}\Omega} = \frac{\hbar m_{\mathrm{e}}(2\pi)^4}{k_i}\left|T_{f,i}\right|^2\rho_{\mathrm{e}}(E_{\mathrm{out}},\Omega)\rho_{\mathrm{v}}(E_{\mathrm{k}}). \tag{9}$$

Note that Eq. (9) differs slightly from the formulas given by Ohlsen [4], Fuchs [5], and Tostevin et al. [6] (used by TT01) since Refs. [4–6] use the alternative momentum normalization

$$\int_{\mathbb{R}^2}\langle \boldsymbol{p}|\boldsymbol{r}\rangle\langle\boldsymbol{r}|\boldsymbol{p}\rangle\,\mathrm{d}\boldsymbol{r} = (2\pi\hbar)^3\delta(\boldsymbol{r}'-\boldsymbol{r}) \tag{10}$$

and hence TT01's Eq. (10) is different from the present Eq. (9) by a factor of $1/(2\pi\hbar)^3$.

We now turn to the evaluation of $\rho_{\mathrm{e}}$ and $\rho_{\mathrm{v}}$. The relationship between continuum-state normalization and density of states can be found in quantum mechanics text such as Cohen-Tannoudji et al. [7]:

$$\int_{[\boldsymbol{\beta}]}\int_0^\infty |\epsilon,\boldsymbol{\beta}\rangle\langle\boldsymbol{\beta},\epsilon|\rho(\epsilon,\boldsymbol{\beta})\,\mathrm{d}\epsilon\,\mathrm{d}\boldsymbol{\beta} = \mathbf{1}, \tag{11}$$

where $\mathbf{1}$ is the identity operator, $\epsilon$ is the continuum-state energy, $\boldsymbol{\beta}$ stands for the set of remaining parameters which characterize the state, and $[\boldsymbol{\beta}]$ is the parameter

space of $\boldsymbol{\beta}$. The scattered electron can be characterized by its energy $E_{\text{out}}$ and direction $\Omega$, and Eq. (11) becomes

$$\int_{\Omega}\int_{0}^{\infty} \langle \boldsymbol{r}'|\boldsymbol{p}\rangle\langle \boldsymbol{p}|\boldsymbol{r}\rangle \rho_{\text{e}}(E_{\text{out}},\Omega)\,\mathrm{d}E_{\text{out}}\,\mathrm{d}\Omega = \delta(\boldsymbol{r}'-\boldsymbol{r}). \quad (12)$$

Substituting $\mathrm{d}\boldsymbol{p} = m_{\text{e}}p\,\mathrm{d}E\,\mathrm{d}\Omega$ into Eq. (6) and comparing with Eq. (12) gives

$$\rho_{\text{e}}(E_{\text{out}},\Omega) = \hbar m_{\text{e}} k_{\text{out}}. \quad (13)$$

For the vibrational continuum we have

$$\int_{0}^{\infty} \nu_{E_{\text{k}}}(R')\nu_{E_{\text{k}}}(R)\rho_{\text{v}}(E_{\text{k}})\,\mathrm{d}E_{\text{k}} = \delta(R'-R). \quad (14)$$

If we use energy-normalized vibrational wave functions (as TT01 have), then the unity resolution

$$\int_{0}^{\infty} \nu_{E_{\text{k}}}(R')\nu_{E_{\text{k}}}(R)\,\mathrm{d}E_{\text{k}} = \delta(R'-R), \quad (15)$$

says that the density of vibrational states is simply

$$\rho_{\text{v}}(E_{\text{k}}) = 1. \quad (16)$$

Finally, substituting Eqs. (13) and (16) into Eq. (9) we obtain

$$\frac{\mathrm{d}^2\sigma}{\mathrm{d}E_{\text{out}}\,\mathrm{d}\Omega} = \hbar^2 m_{\text{e}}^2 (2\pi)^4 \frac{k_{\text{out}}}{k_{\text{in}}} \left|T_{f,i}\right|^2. \quad (17)$$

The relationship between the $T$ matrix and scattering amplitude for various normalizations of the projectile plane waves and relationships between $\mathsf{S}$ and $\mathsf{T}$ can be found in the appendix of Morrison and Sun [8]:

$$T_{fi} = \frac{|c|^2}{d}\frac{\hbar^2}{4\pi m_{\text{e}}} F_{fi}, \quad (18)$$

where the constants $c$ and $d$ are found from

$$\langle \boldsymbol{r}|\boldsymbol{p}\rangle = c(2\pi)^{-3/2} e^{i\boldsymbol{p}\cdot\boldsymbol{r}/\hbar} \quad (19)$$

$$\mathsf{S} = \mathbf{1} + 2id\mathsf{T}. \quad (20)$$

For the momentum-normalized plane waves (4) and the definition $\mathsf{S} = \mathbf{1} - 2\pi i\mathsf{T}$ assumed in Eq. (1) [3] we clearly require

$$c = \frac{1}{\hbar^{3/2}}, \qquad d = \pi, \quad (21)$$

giving:

$$T_{fi} = \frac{1}{(2\pi)^2 i\hbar m_{\text{e}}} F_{fi}, \quad (22)$$

and hence

$$\frac{\mathrm{d}^2\sigma}{\mathrm{d}E_{\text{out}}\,\mathrm{d}\Omega} = \frac{k_{\text{out}}}{k_{\text{in}}} \left|F_{fi}\right|^2. \quad (23)$$

At this point it is evident we have arrived at the expected result that the DDCS is simply given by the standard differential cross section formula.

To express the DDCS in terms of the same partial-wave $T$-matrix elements in TT01's formulas we now directly apply Eqs. (6) and (7) of Malegat [9] to give

$$\frac{\mathrm{d}^2\sigma}{\mathrm{d}E_{\text{out}}\,\mathrm{d}\Omega} = \frac{k_{\text{out}}}{k_{\text{in}}} \left|F_{fi}\right|^2 = \sum_t A^t_{fi} P_t(\cos\theta), \quad (24)$$

where the coefficients $A^t_{fi}$ are given in Malegat's Eq. (8). Note that, according to Malegat's definitions, Eq. (24) is the orientation-averaged DDCS. After integration over the scattered-electron solid angle, we get

$$\begin{aligned}\frac{\mathrm{d}\sigma}{\mathrm{d}E_{\text{out}}} &= 4\pi A^0_{fi} \\ &= \frac{\pi}{k_i^2} \sum_{\substack{\ell' m' \\ \ell m}} \left|\langle \nu_{E_{\text{k}}} | T_{\ell' m', \ell m}(R; E_{\text{in}}) | \nu_v \rangle\right|^2, \end{aligned} \quad (25)$$

where $T_{\ell' m', \ell m}$ are the same partial-wave $T$-matrix elements defined by TT01. The explicit form of $A^0_{f,i}$ can be inferred from TT01 by inspection of their Eq. (29).

[1] C. S. Trevisan and J. Tennyson, J. Phys. B At. Mol. Opt. Phys. **34**, 2935 (2001).
[2] M. C. Zammit, D. V. Fursa, J. S. Savage, and I. Bray, J. Phys. B At. Mol. Opt. Phys. **50**, 123001 (2017).
[3] J. J. Sakurai and J. Napolitano, *Modern Quantum Mechanics* (Addison-Wesley, 2011), 2nd ed.
[4] G. G. Ohlsen, Nucl. Instruments Methods **37**, 240 (1965).
[5] H. Fuchs, Nucl. Instruments Methods Phys. Res. **200**, 361 (1982).
[6] J. A. Tostevin, S. Rugmai, and R. C. Johnson, Phys. Rev. C - Nucl. Phys. **57**, 3225 (1998).
[7] C. Cohen-Tannoudji, B. Diu, and F. Laloe, *Quantum Mechanics. Volume II* (John Wiley and Sons, 1978).
[8] M. A. Morrison and W. Sun, in *Comput. Methods Electron-Molecule Collisions*, edited by W. Huo and F. A. Gianturco (1994).
[9] L. Malegat, Comput. Phys. Commun. **60**, 391 (1990).
